# Supplementary material for: Tractable Compositions of Discrete-Time Control Barrier Functions with Application to Lane Keeping and Obstacle Avoidance
Source: arXiv:2004.01858 source file (2020-04-04)
Supplement: Supplementary file 1 [file sec_appendix.tex]

%!TEX root = main.tex
%\section{Appendix}
\appendix \label{appendix}
